# Supplementary material for: World-Grounded Human Motion Recovery via Gravity-View Coordinates
Source: arXiv:2409.06662 source file (2024-09-10)
Supplement: Supplementary file 1 [file 06_supp.tex]

\section{Details of post-processing}

\subsection{Global translation refinement}
Inspired by WHAM~\cite{wham}, we use joint stationary probabilities to further refine the global motion.
Specifically, we predict the stationary probabilities for the hands, toes, and heels, and then update the global translation frame-by-frame to ensure that the static joints remain at fixed points in space as much as possible.
The algorithm is shown in \AlgRef{alg:pp_traj}.
\begin{algorithm}
    \caption{Global translation refinement}\label{alg:pp_traj}
    \KwIn{Root translations: $\{\tau_i\}_{i=1}^{T}$; Joint positions: $\{\{p^{j}_i\}_{i=1}^{T}\}_{j=1}^{N}$; stationary logits: $\{\{s^{j}_i\}_{i=1}^{T}\}_{j=1}^{N}$}
    \KwOut{Stationary root translations $\{\tau^{*}_i\}_{i=1}^{T}$}
    \For{$i = 1$ \textbf{to} $T$}{
        $\tau^{*}_i \gets \tau_i$;
    }
    \For{$i = 2$ \textbf{to} $T$}{
        $d_i \gets 0$;\\
        \For{$j = 1$ \textbf{to} $N$}{
            $d^j_i \gets (p^{j}_i - p^{j}_{i-1}) * \exp(s^{j}_i) / \sum_{k=1}^{N} \exp(s^{k}_i$);\\
            $ d_i \gets d_i + d^j_i$;
        }
        \For{$k = i$ \textbf{to} $N$}{
            $\tau^{*}_k \gets \tau^{*}_k - d_i$;
        }
        
    }
\end{algorithm}
\subsection{Stationary positions adjustment}
After updating the global translation, we calculate the fine-grained stationary positions for each static joint.
% 这些目标joint positions will then be passed into an inverse kinematics process.
These target joint positions are then passed into an inverse kinematics process to solve the local pose, mitigating physically implausible effects like foot-sliding.
\AlgRef{alg:pp_pose} shows the algorithm.
\begin{algorithm}
    \caption{Stationary positions adjustment}\label{alg:pp_pose}
    \KwIn{Joint positions: $\{p_i\}_{i=1}^{T}$; stationary probabilities: $\{c_i\}_{i=1}^{T}$}
    \KwOut{Stationary joint positions $\{p^{*}_i\}_{i=1}^{T}$}
    \For{$i = 1$ \textbf{to} $T$}{
        $p^{*}_i \gets p_i$;
    }
    \For{$i = 2$ \textbf{to} $T$}{
        $p^{*}_i \gets p^{*}_i \cdot (1 - c_i) + p^{*}_i \cdot c_i$;
    }
\end{algorithm}

\section{Details of training}
\subsection{Training loss}
We use the following losses to train the network.
\begin{align}
    \begin{gathered}
        L_{v}=\|\hat{v_{root}}-v_{root}\|^{2} \\
        L_{GV}=\|\hat{\Gamma_{GV}}-\Gamma_{GV}\|^{2} \\
        L_{\mathrm{SMPL}}=\|\hat{\theta}-\theta\|^{2}+\|\hat{\beta}-\beta\|^{2} \\
        L_{j 3 d}=\|FK(\hat{\theta})-FK(\mathcal{\theta})\|^{2} \\
        L_{j 2 d}=\|\hat{\jmath}-j\|^{2} \\
        L_{v 3 d}=\|\hat{v}-v\|^{2} \\
        L_{s} = BCE(\hat{s}, s)\\
        \end{gathered} 
\end{align}
where $v_{root}$ is the root velocity, $\Gamma_{GV}$ is the global orientation, $\theta$ and $\beta$ are the SMPL parameters in camera coordinates, 
$j$ is the 2D joint position and $v$ is the vertices projected into the full image using the predicted camera parameters similar to~\cite{cliff}.
$FK$ denotes the forward kinematics function and $s$ denotes the joint stationary labels.

\begin{table}
    %\caption{\textbf{Ablation}}
    \centering
    \caption{\textbf{Ablation studies} on the EMDB~\cite{emdb} dataset.}
    % \vspace{-4mm}
    \resizebox{\linewidth}{!}{
        \begin{tabular}{l|ccccccc}
            \toprule
            % Variant & \scriptsize{PA-MPJPE} & \scriptsize{MPJPE} & \scriptsize{Accel} 
            %  & \scriptsize{WA2-MPJPE} & \scriptsize{WAA-MPJPE} & \scriptsize{RTE} & \scriptsize{Jitter} & \scriptsize{Foot-Sliding} \\
            Variant                        & {PA-MPJPE} & {MPJPE}   & {WA-MPJPE} & {W-MPJPE}  & {RTE}    & {Jitter} & {Foot-Sliding} \\
            \midrule
            w/o $GV$                   & 43.2	      & 73.3	 & 642.5	&1231.5	&14.9	&13.8   &23.3          \\
            w/o $\Gamma_{GV}$          & 43.2	      & 81.9	 & 129.1	&366.4	&9.5	&14.6   &\bf{3.4}          \\
            w/o Transformer            & 44.6	      & 83.5	 & 113.2	&283.3	&2.2	&\bf{10.6}	&3.5          \\
            w/o RoPE                   & 107.7	      & 230.9	 & 641.1	&1254.5	&15.3	&30.6   &12.9           \\
            w/o PostProcessing         & 42.7	      & 72.6	 & 119.7	&306.0	&2.9	&16.2   &8.3          \\
            \midrule
            Full Model                 & \bf{42.7}    & \bf{72.6} & \bf{109.1}  & \bf{274.9} & \bf{1.9} & 16.5     & 3.5       \\
            \bottomrule
        \end{tabular}
        \label{tab:ablation_emdb}
    % \vspace{-3mm}
    }
\end{table}

\section{More ablation studies}
In ~\tabref{tab:ablation_emdb}, we conduct ablation studies on the EMDB~\cite{emdb} dataset.
The results on EMDB are similar to RICH. Each of our modules contributes to the final results.

\section{Limitation}
Similar to ~\cite{wham}, our approach cannot handle riding bicycles or skateboards as the training dataset does not have these motions.
Although our method could parallelly process a whole sequence, it might not be suitable for real-time applications.
Moreover, our pipeline does not consider scene geometry which would restrict human motions.

Additionally, while GVHMR achieved significant improvements on the benchmark, challenges remain in providing fine-detailed motion prediction.
For instance, issues like drifting, foot sliding, and jittering persist in difficult sequences.
These challenges are inherent to monocular kinematic-based methods, and we plan to address them in future work.
